# Supplementary material for: TRacer: Scalable Graph-based Transaction Tracing for Account-based Blockchain Trading Systems
Source: arXiv:2201.05757 source file (2022-03-04)
Supplement: Supplementary file 1 [file appendices.tex]

\section{Appendices}

\subsection{Proof of Theorem \ref{thm:run_time}}
\begin{proof}
This follows from Andersen et al. \cite{andersen2006local}, Lemma 2.
\end{proof}

\subsection{Proof of Theorem \ref{thm:push_cost}}
\begin{proof}
The residual of a node $u$ coming from its neighbors ensures that the number of non-zero elements in $R_s(u)$ are less than $|E(u)|$, where $E(u)$ contains edges related to $u$, so the cost of selfPush will not exceed $O(E(u))$.
In addition, forwardPush and backwardPush are both related to the timestamp of edges, so all edges among node $u$ and its neighbors can be sorted according to their timestamp firstly, whose cost is $O(|E(u)|log(|E(u)|))$, and then the summation terms are calculated in a timestamp order, whose cost is $O(|E(u)|)$.
Therefore, the cost of the local push procedure is:
\begin{equation}
    O( |E(u)|log(|E(u)|) + |E(u)| ) = O(|E(u)|log(|E(u)|)).
\end{equation}
\end{proof}

\subsection{Proof of Proposition \ref{pot:ttr_max_height}}
\begin{proof}
In order to maximize the estimate of $\bm{p}_s$ for the nodes having a high order of the source node, $\alpha$ needs to be as small as possible, and $\beta$ needs to be as close as possible to 0 or 1, which ensures that the residual can be pushed to a specific direction.
%  for reducing the dissipation caused by shunting
Considering $\beta=1$ here, the sum of residual pushed from the source node $s$ to the neighbors of order 1 to order $n$ are:
\begin{equation}
    \begin{cases}
        & r^{(1)}=(1-\alpha), \\
        & r^{(2)} \geq (1-\alpha)(r^{(1)}-k_1 \epsilon)=(1-\alpha)^2-(1-\alpha)k_1 \epsilon, \\
        & ...... \\
        & r^{(n)} \geq (1-\alpha)(r^{(n-1)}-k_{n-1} \epsilon) \\
        & \ \ \ \ \ \ \ \ =(1-\alpha)^n-\sum\limits_{i=1}^{n-1}(1-\alpha)^{n-i}k_{n-i} \epsilon, \\
    \end{cases}
\end{equation}
where $k_i$ represents the number of nodes with residual less than $\epsilon$ in the $i$-order neighbors of the source node.
Therefore, $r^{(n)}$ obtains the maximum value when:
\begin{equation}
    \sum\limits_{i=1}^{n-1}(1-\alpha)^{n-i}k_{n-i} \epsilon = 0,
\end{equation}
which means the residual of each $i$-order node greater or equal than $\epsilon$. 
This situation exists when the source node in a path graph, whose adjacency matrix satisfies $A(i,i+1)=1$ and other elements are $0$.
Consider the end condition of the local push procedure, the residual of $n$-order neighbors is:
\begin{equation}
    r^{(n)}=(1-\alpha)^n \leq \epsilon \Rightarrow n \leq \frac{log(\epsilon)}{log(1-\alpha)}.
\end{equation}
\end{proof}

\subsection{Proof of Proposition \ref{pot:ttr_local_comm}}
\begin{proof}
Consider the end condition of TTR-based Local Community Discovery Algorithm:
\begin{equation}
    \Phi(S)=\frac{\bm{p}_s(\partial(S))}{\bm{p}_s(S)} < \varphi,
\end{equation}
and the selfPush procedure at the first iteration of TTR Algorithm ensures:
\begin{equation}
    \bm{p}_s(s) \geq \alpha.
\end{equation}
Since $s \in S$, then $\bm{p}_s(S) \geq \alpha$, so:
\begin{equation}
    \bm{p}_s(\partial(S))<\varphi \alpha,
\end{equation}
which means that the path between $s$ and $v_n$ must be included in the local tracking network when $\bm{p}_s(v_n) \geq \varphi \alpha$. 
In this way, $\bm{p}_s(v_n)$ can obtain a minimum value with only one selfPush operation for $v_n$, and then $\bm{p}_s(v_n) \geq \varphi \alpha$ needs:
\begin{equation}
    % \alpha \sum_t r(v_n)(t) \geq \varphi\alpha \\
% \Rightarrow \sum_t r(v_n)(t) \geq \varphi.
    \alpha ||R_s(v_n)|| \geq \varphi \alpha \Rightarrow ||R_s(v_n)|| \geq \varphi
\label{equ:proof_ttr_local_comm_phi_target}
\end{equation}
Moreover, in order to ensure that at least one selfPush operation on $v_n$, the residual of $v_n$ must be greater than $\epsilon$, that is:
\begin{equation}
    \varphi \geq \epsilon.
\end{equation}
Consider that satisfying Equation \ref{equ:proof_ttr_local_comm_phi_target} in the worst case: 
1) The path between the source node and a target node is weakly connected, which makes the tracking tendency invalid.
2) The edges related to each node on the paths among the source node and the target node have the same weight, which makes the weight pollution invalid. 
3) Each path between the source node and a target node without increasing or decreasing timestamp, which makes time reasoning invalid.
4) There is only one path between the source node and a target node.
In this case, in order to satisfy the Equation \ref{equ:proof_ttr_local_comm_phi_target}, the residual sum of $m$-order neighbors ($m \leq n$) of the target node $v_n$ are:
\begin{equation}
    \begin{cases}
        & r^{(n)} \geq \varphi, \\
        & r^{(n-1)} \geq \frac{\varphi d_{n-1}}{min(\beta,1-\beta)(1-\alpha)}, \\
        & r^{(n-2)} \geq \frac{\varphi d_{n-1}d_{n-2}}{min^2(\beta,1-\beta)(1-\alpha)^2}, \\
        & ......\\
        & r^{(n-m)} \geq \frac{\varphi \prod\limits_{i=1}^{m}d_{n-i}}{min^m(\beta,1-\beta)(1-\alpha)^m},
    \end{cases}
\end{equation}
where $d_{n-i}$ denotes the degree of the $n-i$ order node in this path.
Consider the inequality as follow:
\begin{equation}
    \prod\limits_{i=1}^{m}d_{n-i} \leq (\frac{1}{m}\sum\limits_{i=1}^{m}d_{n-i})^m \rightarrow \bar{d}^m.
\end{equation}
If the $m$-order neighbor of the target node is the source node, then:
\begin{equation}
    1 \geq \frac{\varphi \bar{d}^n}{min^n(\beta,1-\beta)(1-\alpha)^n}
\Rightarrow \bar{d}\varphi^{\frac{1}{n}} \leq (1-\alpha) \cdot min(\beta,1-\beta)
\end{equation}
\end{proof}
